# Supplementary material for: Newton-ADMM: A Distributed GPU-Accelerated Optimizer for Multiclass Classification Problems
Source: arXiv:1807.07132 source file (2020-02-04)
Supplement: Supplementary file 1 [file appendix.tex]

\section{More Details On Softmax Function~\eqref{eq:softmax_log_likelihood}}
\subsection{Relationship to Logistic Regression with $ \pm1 $-labels}
\label{sec:logistics_pm1}
Sometimes, in the literature, for the two-class classification problem, instead of $ \{0,1\} $ the labels are marked as $ \pm1 $. In this case, the corresponding logistic regression is written as
\begin{align*}
&F(\xx)  = \sum_{i=1}^{n} \log \left( 1+e^{-b_{i} \xx^{T} \aa_{i} } \right).
\end{align*}
In this case, we have
\begin{align*}
&F(\xx) = \sum_{i=1}^{n} \log \left( e^{\frac{- \xx^{T} \aa_{i}}{2}} + e^{\frac{\xx^{T} \aa_{i}}{2}} \right) - \frac{b_{i} \xx^{T} \aa_{i}}{2} \\
&= \sum_{i=1}^{n} \log \left(e^{\frac{- \xx^{T} \aa_{i}}{2}} \left( 1 + e^{\xx^{T} \aa_{i}} \right) \right) - \frac{b_{i} \xx^{T} \aa_{i}}{2} \\
&= \sum_{i=1}^{n} \log \left( 1 + e^{\xx^{T} \aa_{i}} \right) - \frac{(1+b_{i}) \xx^{T} \aa_{i}}{2} \\
&= \sum_{i=1}^{n} \log \left( 1 + e^{\xx^{T} \aa_{i}} \right) - \tilde{b}_{i} \xx^{T} \aa_{i},
\end{align*}
where $ \tilde{b}_{i} \in \{0,1\} $. Hence this formulation co-incides with~\eqref{eq:softmax_log_likelihood}. 
%In fact, since we assumed that $ b \in \mathbb{R} $, we can give it any label we want, we still get~\eqref{eq:softmax_log_likelihood}. 

\subsubsection{Softmax Multi-Class problem is (strictly) convex}
\label{sec:softmax_convex}
Consider the data matrix $X \in \mathbb{R}^{n \times d}$ where each row, $\aa_{i}^{T}$, is a row vector corresponding to the $i^{th}$ data point. The Hessian matrix can be written as
\begin{align*}
\nabla^{2} \mathcal{L} = \mathbf{X}^{T} \mathbf{W} \mathbf{X},
\end{align*}
where
\begin{align*}
\mathbf{X} &= \begin{bmatrix}
X & 0  & \ldots & 0 \\
0& X  & \ldots & 0 \\
\vdots & & \ddots & \vdots \\
0& 0  & \ldots & X
\end{bmatrix}_{(n\times (C-1)) \times (d \times (C-1))}, \\
\mathbf{W} &= \begin{bmatrix}
W_{1,1} & W_{1,2}  & \ldots & W_{1,C-1} \\
W_{2,1}& W_{2,2}  & \ldots & W_{2,C-1} \\
\vdots & & \ddots & \vdots \\
W_{C-1,1}& W_{C-1,2}  & \ldots & W_{C-1,C-1}
\end{bmatrix},
\end{align*}
and each $W_{c,c}$ and $W_{c,b}$ is a $n \times n$ diagonal matrix corresponding to~\eqref{eq:softmax_hessian_wc_wc} and~\eqref{eq:softmax_hessian_wc_wb}, respectively. 
Note that since 
\begin{align*}
&\left(\frac{e^{\lin{\aa_{i}, \xx_{c}}}}{1+\sum_{c' = 1}^{C-1} e^{\lin{\aa_{i}, \xx_{c'}}}} - \frac{e^{2\lin{\aa_{i}, \xx_{c}}}}{\left(1+\sum_{c' = 1}^{C-1} e^{\lin{\aa_{i}, \xx_{c'}}}\right)^{2}} \right) - \\
&\sum_{\substack{b = 1 \\ b \neq c}}^{C-1} \frac{e^{\lin{\aa_{i}, \xx_{\hat{c}} + \xx_{c}}}}{\left(1+\sum_{c' = 1}^{C-1} e^{\lin{\aa_{i}, \xx_{c'}}}\right)^{2}} \\
& = \left(\frac{e^{\lin{\aa_{i}, \xx_{c}}}}{1+\sum_{c' = 1}^{C-1} e^{\lin{\aa_{i}, \xx_{c'}}}} - \frac{e^{2\lin{\aa_{i}, \xx_{c}}}}{\left(1+\sum_{c' = 1}^{C-1} e^{\lin{\aa_{i}, \xx_{c'}}}\right)^{2}} \right) \\
&  \quad \quad  - \frac{e^{\lin{\aa_{i}, \xx_{c}}}}{1+\sum_{c' = 1}^{C-1} e^{\lin{\aa_{i}, \xx_{c'}}}} \left( \sum_{\substack{b = 1 \\ b \neq c}}^{C-1}  \frac{e^{\lin{\aa_{i}, \xx_{\hat{c}} }}}{1+\sum_{c' = 1}^{C-1} e^{\lin{\aa_{i}, \xx_{c'}}}} \right) \\
& = \left(\frac{e^{\lin{\aa_{i}, \xx_{c}}}}{1+\sum_{c' = 1}^{C-1} e^{\lin{\aa_{i}, \xx_{c'}}}} - \frac{e^{2\lin{\aa_{i}, \xx_{c}}}}{\left(1+\sum_{c' = 1}^{C-1} e^{\lin{\aa_{i}, \xx_{c'}}}\right)^{2}} \right) \\
&  \quad  \quad - \frac{e^{\lin{\aa_{i}, \xx_{c}}}}{1+\sum_{c' = 1}^{C-1} e^{\lin{\aa_{i}, \xx_{c'}}}} \left( 1-\frac{1 + e^{\lin{\aa_{i},\xx_{c}}}}{1+\sum_{c' = 1}^{C-1} e^{\lin{\aa_{i}, \xx_{c'}}}}  \right) \\
& = \frac{e^{\lin{\aa_{i}, \xx_{c}}}}{\left(1+\sum_{c' = 1}^{C-1} e^{\lin{\aa_{i}, \xx_{c'}}}\right)^{2}} > 0,
\end{align*}
the matrix $\mathbf{W}$ is strictly diagonally dominant, and hence it is symmetric positive definite. So the problem is convex (in fact it is strictly-convex if the data matrix $ \vec{A} $ is full column rank).

\section{Tensorflow's Performance Comparison on Various Compute Platforms}
\label{sec:platform-cpu-gpu}
\begin{table}[!htb]
\centering
\caption{Performance comparison between first-order and second-order methods on CPU-only and 1-GPU-1-CPU-core compute platforms
for \textit{covertype} dataset. 
Batch-size 128 first order methods are compared with second order methods using full gradient and hessian sample size set to 5\%. 
Batch-size 20\% first order methods are compared with second order methods using sample sizes of 20\% and 5\% for gradient 
and hessian computations respectively. } 
\label{table-cpu-gpu-comparison}
\scalebox{0.9}{
\begin{tabular}
      {cccc} \hline 
      Time vs. Accuracy & Time vs. Misfit  & Time vs. Accuracy & Time vs. Misfit \\
      \multicolumn{2}{c}{Batch Size = 128} & \multicolumn{2}{c}{Batch Size = 20\%} \\       
       \multicolumn{2}{c}{Gradient Sample Size = 100\%} & \multicolumn{2}{c}{Gradient Sample Size = 20\%} \\       
      \multicolumn{2}{c}{Hessian Sample Size = 5\%} & \multicolumn{2}{c}{Hessian Sample Size = 5\%} \\       
	\hline
      \multicolumn{4}{c}{  	\parbox[c]{6in}{
      	\includegraphics[width=6in, height=0.5in]{./figures-uniform-cpu/uniform_legend.pdf}
      } }	\\
 	\parbox[c]{1.5in}{
      	\includegraphics[width=1.4in, height=1.1in]{./figures-uniform-cpu/normalized_batch-128_forest_time_test_accuracy_5_100_10.pdf}
      } & 
 	\parbox[c]{1.5in}{
      	\includegraphics[width=1.4in, height=1.1in]{./figures-uniform-cpu/normalized_batch-128_forest_time_train_function_5_100_10.pdf}
      } & 
 	\parbox[c]{1.5in}{
      	\includegraphics[width=1.4in, height=1.1in]{./figures-uniform-cpu/normalized_batch-20_forest_time_test_accuracy_5_20_10.pdf}
      } & 
 	\parbox[c]{1.5in}{
      	\includegraphics[width=1.4in, height=1.1in]{./figures-uniform-cpu/normalized_batch-20_forest_time_train_function_5_20_10.pdf}
      } \\
      \multicolumn{4}{c}{Using CPU-only cores for Tensorflow implementations. Newton-type methods use 1-GPU-1-CPU-core.} \\      
      \multicolumn{4}{c}{} \\      
      \multicolumn{4}{c}{} \\      
 	\parbox[c]{1.5in}{
      	\includegraphics[width=1.4in, height=1.1in]{./figures-uniform-gpu/normalized_batch-128_forest_time_test_accuracy_5_100_10.pdf}
      } & 
 	\parbox[c]{1.5in}{
      	\includegraphics[width=1.4in, height=1.1in]{./figures-uniform-gpu/normalized_batch-128_forest_time_train_function_5_100_10.pdf}
      } & 
 	\parbox[c]{1.5in}{
      	\includegraphics[width=1.4in, height=1.1in]{./figures-uniform-gpu/normalized_batch-20_forest_time_test_accuracy_5_20_10.pdf}
      } & 
 	\parbox[c]{1.5in}{
      	\includegraphics[width=1.4in, height=1.1in]{./figures-uniform-gpu/normalized_batch-20_forest_time_train_function_5_20_10.pdf}
      } \\
      \multicolumn{4}{c}{Using 1-GPU-1-CPU-core for Tensorflow implementations. Newton-type methods use 1-GPU-1-CPU-core.} \\            
      \multicolumn{4}{c}{} \\      
      \multicolumn{4}{c}{} \\      \hline
\end{tabular}
}
\end{table}

%
% Discussion and Analysis of different compute platforms
%

Columns 1 and 2 of table~\ref{table-cpu-gpu-comparison} plots the results for~\textit{covertype} dataset,
when batch size is set to 128, using CPU-only cores (row 1) and 1-GPU-1-CPU-core (row 2) for first-order 
tensorflow implementations. Note that newton-type methods always use 1-GPU-1-CPU-core as the 
compute platform irrespective of any of the hyper-parameter settings. We clearly notice that the first-order 
methods takes $ \approx $ 600 seconds when GPU cores are used compared to $ \approx $
350 seconds when CPU cores are used. This can be attributed to the small batch size used for first-order
methods. Smaller batch size results in computing the gradient, a compute-intensive operation, much more
frequently compared to a large batch size. For the plots shown in table~\ref{table-cpu-gpu-comparison} 
training size for ~\textit{covertype} is set to 450,000. This means gradient is computed $ \approx $ 3516
times to complete each of the training epochs in this instance. Since the batch size is very small most
of the GPU cores are idle during every computation of the gradient resulting in low GPU occupancy (which 
is the ratio of active warps on an SM and maximum allowed warps). Also 
with each invocation of gradient computation there is CUDA kernel instantiation overhead which accumulates
as well. Because of above reasons small batch sizes yield high time per epoch for first-order methods. 

Columns 3 and 4 of table~\ref{table-cpu-gpu-comparison} plots for the results for \textit{covertype} dataset
using a large batch size, of 20\% of the dataset. Note that batch size for first-order methods is same as the 
gradient sample size for newton-type methods for these plots. We clearly notice that first-order tensorflow
methods takes $ \approx $ 55 seconds when CPU-only cores are used as the compute platform
compared to $ \approx $ 22.5 seconds when 1-GPU-1-CPU-core is used, a speedup of $2 \times$ over
CPU only compute platform. In this instance, during each epoch of first-order methods gradient is evaluated
only 5 times. Because of the large batch size, $ \approx $ 90,000 points, are processed by the GPU resulting
in higher utilization of the GPU cores (compared to the same computation using smaller batch size). 
This explains why GPU-cores yield shorter time per epoch when large
batch size are used for first-order methods.
